# Supplementary material for: Towards Rationality in Language and Multimodal Agents: A Survey
Source: arXiv:2406.00252 source file (2025-02-16)
Supplement: Supplementary file 1 [file appendix.tex]

\newpage
\appendix
\onecolumn
\section{Orderability of Preferences.}
\label{sec: orderability}
\paragraph{Comparability} When faced with any two alternatives A and B, the agent should have at least a weak preference, i.e., $A \succeq B$ or $B \succeq A$. This means that the agent can compare any pair of alternatives and determine which one is preferred or if they are equally preferred.
\paragraph{Transitivity} If the agent prefers A to B and B to C, then the agent must prefer A to C. This ensures that the agent's preferences are consistent and logical across multiple comparisons.
\paragraph{Closure} If A and B are in the alternative set S, then any probabilistic combination of A and B (denoted as ApB) should also be in S. This principle ensures that the set of alternatives is closed under probability mixtures.
\paragraph{Distribution of probabilities across alternatives} If A and B are in S, then the probability mixture of (ApB) and B, denoted as [(ApB)qB], should be indifferent to the probability mixture of A and B, denoted as (ApqB). This principle ensures consistency in the agent's preferences when dealing with probability mixtures of alternatives.
\paragraph{Solvability} When faced with three alternatives A, B, and C, with the preference order $A \succeq B \succeq C$, there should be some probabilistic way of combining A and C such that the agent is indifferent between choosing B or this combination. In other words, the agent should be able to find a solution to the decision problem by making trade-offs between alternatives.
\\ 
\\
One consequence of the orderability is the concept of \textbf{dominance}: If alternative A is better than alternative B in terms of one attribute and at least as good in terms of all other attributes, the dominant option A should be chosen. An example of a fallacy that violates dominance is the sunk cost fallacy, where an agent continues to invest in a suboptimal alternative due to past investments, despite the availability of better options based on future outcomes.

\section{Information Grounding}
\label{sec: Information Grounding}
Web agents are a quintessential example of how multi-modal agents surpass language-only ones. In agents like Pix2Act~\cite{shaw2024pixels}, WebGUM~\cite{furuta2023multimodal}, CogAgent\cite{hong2023cogagent}, and SeeAct~\cite{zheng2024gpt}, web navigation is grounded on graphical user interface (GUI) rather than solely on HTML texts~\cite{shen2024small, yao2022webshop, deng2024mind2web, gur2023real}. This method of visual grounding offers higher information density compared to HTML codes that are usually lengthy, noisy, and sometimes even incomplete~\cite{zheng2024gpt}. Supporting the importance of vision, ablation studies in WebGUM~\cite{furuta2023multimodal} also reports $5.5\%$ success rate improvement on the MiniWoB++ dataset~\cite{shi2017world, liu2018reinforcement} by simply adding the image modality.

Multi-modalities also help enhance the functionality of agent systems through more diverse information grounding. For example, Chain-of-Action~\cite{pan2024chain} advances the single-modal Search-in-the-Chain~\cite{xu2023search} by supporting multi-modal data retrieval for faithful question answering. DoraemonGPT~\cite{yang2024doraemongpt} decomposes complex tasks into simpler ones toward understanding dynamic scenes, where multi-modal understanding is necessary for spatial-temporal videos analysis. RA-CM3~\cite{yasunaga2022retrieval} augments baseline retrieval-augmented LLMs with raw multi-modal documents that include both images and texts, assuming that these two modalities can contextualize each other and make the documents more informative, leading to better generator performance. The multi-modal capabilities also allow HuggingGPT~\cite{shen2024hugginggpt}, Agent LUMOS~\cite{yin2023lumos}, ToolAlpaca~\cite{tang2023toolalpaca}, and AssistGPT~\cite{gao2023assistgpt} to expand the scope of tasks they can address, including cooperation among specialized agents or tools capable of handling different information modalities.

Large world models is an emerging and promising direction to reduce multi-modal hallucinations. The notion is also mentioned in ``Objective-driven AI"~\cite{lecun2024deep}, where agents have behavior driven by fulfilling objectives and they understand how the world works with common sense knowledge, beyond an auto-regressive generation. %\citet{lecun2024deep} proposes the urgency for agents to learn to reason beyond feed-forward, i.e., the System 1 subconscious computation, and start making System 2 reasoning and planning on complicated actions to satisfy objectives with a grounding on world models. 
For example, Large World Model (LWM)~\cite{liu2024world} and Sora~\cite{videoworldsimulators2024} develop insights from both textual knowledge and the world through video sequences. Although these models both advance toward general-purpose simulators of the world, they still lack reliable physical engines for guaranteed grounding in real-world dynamics. Ghost-in-the-Minecraft~\cite{zhu2023ghost} and Voyager~\cite{wang2023voyager} have agents living in a well-defined game-world environment. JEPA~\cite{lecun2022path} creates a recurrent world model in an abstract representation space.

\section{Knowledge Retrieval \& Tool Usage}
\label{sec: Knowledge Retrieval}
Compared to language-only models, MAVEx~\cite{wu2022multi} improves system's scores by $9.5\%$ compared to an image-only baseline through the integration of knowledge from ConceptNet~\cite{speer2017conceptnet} and Wikipedia~\cite{wiki}. It also improves the scores by $8.3\%$ by using the image modality for cross-modal validations with an oracle. Thanks to the external knowledge base, ReAct~\cite{yao2022react} reduces false positive rates from hallucination by $8.0\%$ compared to CoT~\cite{wei2022chain}. CuriousLLM~\cite{yang2024curiousllm} presents ablation studies showing the effectiveness of KGs on improving reasoning within the search process. MineDojo~\cite{fan2022minedojo} observes that internet-scale multi-modal knowledge allows models to significantly outperform all creative task baselines. Equipped with world knowledge, RA-CM3~\cite{yasunaga2022retrieval} can finally generate faithful images from captions compared to CM3~\cite{aghajanyan2022cm3} and Stable Diffusion~\cite{rombach2022high}. CooperKGC~\cite{ye2023beyond} enables multi-agent collaborations, leveraging knowledge bases of different experts. It finds that the incorporation of KGs improves F1 scores by $10.0$-$33.6\%$ across different backgrounds, and adding more collaboration rounds also enhance performance by about $10.0$-$30.0\%$. DoraemonGPT~\cite{yang2024doraemongpt} supports knowledge tools to assist the understanding of specialized video contents. SIRI~\cite{wang2023towards} builds a multi-view knowledge base to increase the explainability of visual question answering.

A multi-agent system can coordinate agents understanding when and which tool to use, which modality of information the tool should expect, how to call the corresponding API, and how to incorporate outputs from the API calls, which anchors subsequent reasoning processes with more accurate information beyond their parametric memory. For example, VisProg~\cite{gupta2023visual}, ViperGPT~\cite{suris2023vipergpt}, and Parsel~\cite{zelikman2023parsel} generate Python programs to reliably execute subroutines. \citet{gupta2023visual, suris2023vipergpt} also invoke off-the-shelf models for multimodal assistance.

Foundation models are not specifically trained for object detection or segmentation, so BuboGPT~\cite{zhao2023bubogpt} and Multi-Agent VQA~\cite{jiang2024multi} call SAM~\cite{kirillov2023segany, ren2024grounded} as the tool.
% \xw{this sentence is a run-on. should probably break it into two sentence.}
% MemGPT~\cite{packer2023memgpt} utilizes different storage tiers to provide extended contexts and turns LLMs into Operating Systems with more rational data flows. Besides, 
Besides, BabyAGI~\cite{nakajima2023babyagi}, Chamelon~\cite{lu2024chameleon}, AssistGPT~\cite{gao2023assistgpt}, Avis~\cite{hu2024avis}, ToolAlpaca~\cite{tang2023toolalpaca}, MetaGPT~\cite{hong2023metagpt}, Agent LUMOS~\cite{yin2023lumos}, AutoAct~\cite{qiao2024autoact}, $\alpha$-UMi~\cite{shen2024small}, and ConAgents~\cite{shi2024learning} harness compositional reasoning to enable generalized multi-agent systems with planning and modular tool-using capabilities in real-world scenarios.

In most cases, tools require translating natural language queries into API calls with predefined syntax. Once the APIs and their input arguments are determined, the tools will ignore any irrelevant context in the original queries, as long as the queries share the same underlying logic necessary for the inputs. Take Multi-Agent VQA~\cite{jiang2024multi} as an example. In this system, a language model provides only the relevant object names to the Grounded SAM~\cite{ren2024grounded} component, which functions as an object detector, rather than passing the entire visual question. Similarly, the image editing tools in VisProg~\cite{gupta2023visual} only receive a fixed set of arguments translated from user queries to perform deterministic code executions. SeeAct~\cite{zheng2024gpt} as a Web agent explores vision-language models, ranking models, and a bounding box annotation tool to improve Web elements grounding from lengthy and noisy HTML codes. 

\section{Collective Deliberation among Agents}
\label{sec: Collective Deliberation}
\subsection{More Examples on Multi-Agent Collaborations}\label{app_collab}
DyLAN~\cite{liu2023dynamic} implements an agent importance scores to optimizes aggregated information from multiple agents. Corex~\cite{sun2023corex} finds that orchestrating multiple agents to work together yields better complex reasoning results, exceeding strong single-agent baselines~\cite{wang2022self} by an average of $1.1$-$10.6\%$. 
Retroformer~\cite{yao2023retroformer} equips the single-agent Reflexion~\cite{shinn2024reflexion} algorithm with an additional LLM to generate verbal reinforcement cues and assist its self-improvement, enhancing accuracy by $1.0$-$20.9\%$. 
MetaAgents~\cite{li2023metaagents} effectively coordinate agents within task-oriented social contexts to achieve consistent behavior patterns, and the implementation of agent reflection in this system leads to a $21.0\%$ improvement in success rates. Multi-agent debating in \citet{khan2024debating} also leads to more truthful answers, boosting single-agent baselines by $28.0\%$.
Multi-Agent Collaboration~\cite{talebirad2023multi}, ChatDev~\cite{qian2023communicative}, AgentCF~\cite{zhang2023agentcf}, AutoGen~\cite{wu2023autogen}, Social Learning~\cite{mohtashami2023social}, S$^{3}$~\cite{gao2023s}, \citet{ke2024enhancing}, and \citet{chern2024combating} continue to push the frontier of a multi-agent system's applications beyond daily conversation to a versatile set of real-world task completions.

\subsection{Collaboration Againt Jailbreaking}\label{app_jail}
LLMs are also sensitive to prompt perturbations due to token bias and noises~\cite{sclar2023quantifying}. One of the most worrying examples are adversarial attacks~\cite{gehman2020realtoxicityprompts, ganguli2022red, du2022ppt, wei2024jailbroken, perez2022red, zou2023universal} through malicious prompt engineering. These attacks, also known as the Red Team Task, also named the Red Team Task, involve malicious prompt engineering designed to exploit vulnerabilities in the model. To combat this issue, \citet{chern2024combating} propose a multi-agent debating approach involving agents with harmless, neutral, or harmful intentions. The authors demonstrate that engaging these agents in multi-round, multi-agent debate is more effective in improving the model's robustness against adversarial prompt variations and perturbations compared to a single-agent with self-reflection prompts. 

\subsection{Collaboration on LLM-based Evaluation}\label{app_multi_eval}
LLM-based evaluation methods are popular in assessing open-ended language responses. \citet{stureborg2024large, koo2023benchmarking} point out LLMs often present cognitive biases in their evaluations, favoring certain types of responses over others regardless of the actual quality or relevance of the respective responses. To establish a more coherent preference orderability aligned with human preference.
ChatEval~\cite{chan2023chateval} introduces a multi-agent debate framework to mimic human annotators collaborating in robust answer evaluations. Its multi-agent approach achieves greater alignment with human preferences compared to single-agent evaluations, enhancing accuracy by $6.2\%$ for GPT-3.5 and $2.5\%$ for GPT-4, and an increase of $16.3\%$ and $10.0\%$ in average Spearman and Kendall-Tau correlations~\cite{zhong2022towards} with human judgements in GPT-4.

\subsection{The Orderability of Preferences Matters for LLM-based Evaluations}\label{sec:app_llm_eval}
This section talks about LLM-based evaluation rather than evaluating the rationality of LLMs discussed in Section~\ref{sec:eval}. Recent research underscores a critical need for more rational LLM-based evaluation methods, particularly for assessing open-ended language responses.  CoBBLEr~\cite{koo2023benchmarking} provides a cognitive bias benchmark for evaluating LLMs as evaluators, revealing a preference for their own outputs over those from other LLMs. \citet{stureborg2024large} argues that LLMs are biased evaluators towards more familiar tokens and previous predictions, and exhibit strong self-inconsistency in the score distribution. \citet{luo2023chatgpt, shen2023large, gao2023human, wang2023chatgpt, chen2023exploring, chiang2023closer, zheng2024judging, fu2023gptscore, liu2023gpteval} also point out the problem with a single LLM as the evaluator, with concerns over factual and rating inconsistencies, a high dependency on prompt design, a low correlation with human evaluations, and struggles with the comparison. As a result, having a coherent orderability of preferences aligned with human preference becomes increasingly important.

Multi-agent systems might be a possible remedy. By involving multiple evaluative agents from diverse perspectives, it becomes possible to achieve a more balanced and consistent orderability of preferences. For instance, ChatEval~\cite{chan2023chateval} posits that a multi-agent debate evaluation usually offers judgments that are better aligned with human annotators compared to single-agent ones.
\citet{bai2024benchmarking} also finds decentralized methods yield fairer evaluation results.

\section{Neuro-Symbolic Reasoning}
\label{sec: Neuro-Symbolic Reasoning} Logic-LM~\cite{pan2023logic} combines problem formulating, symbolic reasoning, and result interpreting agents, where the symbolic reasoner empowers LLMs with deterministic symbolic solvers to perform inference, ensuring a correct answer is consistently chosen. Its multi-agent framework also encourages self-refinement that modifies logical formulation errors using error messages from the symbolic reasoner as the feedback.
% improving accuracy by $0.1$-$2.6\%$ across datasets. 
Besides, SymbolicToM~\cite{sclar2023minding} and KRISP~\cite{marino2021krisp} construct explicit symbolic graphs and answer questions by retrieving nodes in the graph. 
% Binder~\cite{cheng2022binding}, Parsel~\cite{zelikman2023parsel}, LEFT~\cite{hsu2024s}, and \citet{fang2024large} parse input queries and decompose tasks to symbolic modules, which help maintain a coherent order of preferences among the symbolic options in their outputs. 
Binder~\cite{cheng2022binding}, Parsel~\cite{zelikman2023parsel}, LEFT~\cite{hsu2024s}, and \citet{fang2024large} decompose tasks into planning, parsing, and execution, where the symbolic reasoning agents can help maintain a coherent order of preferences among symbolic options in the system outputs. 

\section{Evaluating Rationality}
\subsection{Benchmarks for Hallucination}
\label{sec: Benchmarks for Hallucination}
Multiple evaluation benchmarks targeting language-only dialogue have been proposed, such as BEGIN~\cite{dziri2022evaluating}, HaluEval~\cite{li2023halueval}, DialFact~\cite{gupta2021dialfact}, FaithDial~\cite{dziri2022faithdial}, AIS~\cite{rashkin2023measuring}, and others~\cite{zheng2023does, das2023diving, cao2021hallucinated}. In contrast, \textit{benchmarks on multi-agent frameworks beyond language dialogue or those involving multi-modalities are very limited.} \citet{liu2024exploring} moves beyond conversation to code generation; EureQA~\cite{li2023deceiving} focuses on reasoning chains; and TofuEval~\cite{tang2024tofueval} evaluates hallucination in multi-domain summarization. Object hallucination~\cite{rohrbach2018object, biten2022let}, POPE~\cite{li2023evaluating}, and LLaVA-RLHF~\cite{sun2023aligning} are the few examples evaluating multi-modal hallucination.

\subsection{Perturbation Techniques}
\label{sec: Perturbation Techniques}
Perturbation techniques typically involve some versions of paraphrasing or permutation. Paraphrasing includes changing the instruction templates \cite{weber2023mind}, rewording task descriptions \citep{yang2023rethinking, ohmer2024form, wang2024benchmark}, translating the prompts into a different language \citep{ohmer2023separating, ohmer2024form, xu2024exploring} and then back to the original language \cite{yang2023rethinking}, and making subtle changes to entities in task descriptions without affecting the logical structure, like altering names of the characters, numerical values in math problems, or locations of the events \cite{wang2024benchmark}. Permutation also includes reordering in-context learning examples \cite{lu2021fantastically, pecher2024sensitivity} and, in the case of multiple-choice questions, rearranging the options \citep{zong2023fool, zheng2023large}.
